# Supplementary material for: Parameterizing Activation Functions for Adversarial Robustness
Source: arXiv:2110.05626 source file (2021-10-11)
Supplement: Supplementary file 1 [file additional_statements.tex]

\section{Reproducibility Statement}
To ensure reproducibility, we have provided details on experimental setup in Appendix \ref{app:experimental_setup}. Additionally, we have provided our code in the supplementary.
